# Supplementary material for: Vote'n'Rank: Revision of Benchmarking with Social Choice Theory
Source: arXiv:2210.05769 source file (2023-02-12)
Supplement: Supplementary file 1 [file appendix_rules.tex]

\section{Vote'n'Rank's Procedures}
\textbf{Scoring rules}. Consider the vector of scores $(s_1, \ldots, s_k, \ldots, s_m)$ where $s_k$ is the score of the alternative that is at the place $k$ of any criterion. Let $s_{ij}$ be the score of the alternative $i$ in the criterion $j$. Then the total score of each alternative is calculated as the sum of corresponding scores in each criterion $S_i=\sum_{j=1}^n {s_{ij}}$. The alternatives with the highest scores form the final decision. We study the following rules that differ in scoring vectors.
    \begin{enumerate}
        \item \textit{Plurality rule} $(1,0,\ldots,0)$
        \item \textit{2-Approval rule} $(1,1,0,\ldots,0)$
        \item \textit{Antiplurality rule} $(1,\ldots,1,0)$
        \item \textit{Borda rule} $(m-1,m-2,\ldots,1,0)$
    \end{enumerate}
\textbf{Scoring elimination rules}. After the total score is calculated the alternative with the lowest score is eliminated until we get one or many alternatives with the same score. We study the following scoring elimination rules.
    \begin{enumerate}
        \item \textit{Hare rule} $(1,0,...,0)$
        \item \textit{Baldwin rule} $(m-1,m-2,...,1,0)$
    \end{enumerate}
\textbf{Other positional rules}. The next 3 rules are modifications of the rules above.
    \begin{enumerate}
        \item \textit The {Threshold rule} is similar to the Antiplurality rule, but when there are ties then the new scoring vector $(1,1,...1,0,0)$ is considered to compare tied alternatives. The algorithm stops when it is impossible to break ties.  
        \item \textit The {Coombs rule} considers the scoring vector $(1,0,...,0)$ at first. If there is an alternative that has a simple majority ($S_i>m/2$), then it is the final decision. Else the algorithm uses the Scoring elimination for the scoring vector $(1,...,1,0)$
        \item \textit The {Nanson rule}. The algorithm uses the scoring vector $(m-1,m-2,...,1,0)$ to calculate total scores. Then it  calculates average score $\overline{S}=\sum_{j=i}^m {S_{i}}/m$ and eliminates all alternatives with $S_i<\overline{S}$. The algorithm stops when no more alternatives can be eliminated.
        \item \textit{Black rule}. If the Condorcet winner (the alternative that wins over any other by majority of criteria in pairwise comparison) exists, then it is the final decision. Otherwise, the Borda rule is used.
    \end{enumerate}
\textbf{Majority-relation based rules}. Let's define a majority relation $\mu$ over the set of alternatives as the following binary relation: $a \mu b$ if and only if $a$ is ranked higher than $b$ by more criteria. We present here the rules following definitions from \cite{10.1007/978-3-319-59421-7_8}. The properties of those rules are studied in \cite{Subochev2010}.
    \begin{enumerate}
        \item The \textit{Minimal dominant set}. A set Q is called a dominant set if each alternative in Q dominates each alternative outside Q via $\mu$. A minimal dominant set or the union of these sets is the final decision.
        \item \textit The {Minimal undominated set}. A set Q is called an undominated set if no alternative outside Q dominates any alternative in Q via $\mu$. A minimal undominated set or the union of these sets is the final decision.
        \item The \textit{Uncovered set I}. Define the lower counter set of alternative $a$ as the set of alternatives dominated by $a$ via $\mu$: $L(a)=\{x\in A,a \mu x\} $. Let's construct a new binary relation $\delta_1$: $a \delta_1 b \leftrightarrow L(a) \supset L(b) $. The undominated alternatives via $\delta_1$ are chosen.
        \item The \textit{Uncovered set II}. Define the upper counter set of alternative $a$ as the set of alternatives that dominate $a$ via $\mu$: $U(a)=\{x\in A,x \mu a\} $. Let's construct a new binary relation $\delta_2$: $a \delta_2 b \leftrightarrow a \mu b$ and $U(a) \subseteq  U(b) $. The undominated alternatives via $\delta_2$ are chosen.
        \item \textit{Richelson's rule}. Construct a new binary relation $\delta_3$: $a \delta_3 b \leftrightarrow [L(a) \supseteq L(b) \wedge U(a) \subseteq  U(b) \wedge [L(a) \supset L(b) \vee  U(a) \subset  U(b) ] ]$. The undominated alternatives via $\delta_3$ are chosen.
        \item The \textit{Minimal weakly stable set}. A set  Q  is called a weakly stable set if and only if it satisfies the following property: if for  $x \in Q$  $y \mu x$  holds for some $y$, then either  $y \in Q$  or $ \exists z  \in Q$ s.t. $z \mu y $ 
        \item \textit{Fishburn's Rule}. Construct a new binary relation $\delta_4$: $a \delta_4 b \leftrightarrow U(a) \subset  U(b) $. The undominated alternatives via $\delta_4$ are chosen.
        \item \textit{Copeland's rule I}. Define $u(x)=|L(x)|-|U(x)|$. The final decision is formed by the alternatives with the highest $u(x)$.
        \item \textit{Copeland's rule II}. Define $u(x)=|L(x)|$. The final decision is formed by the alternatives with the highest $u(x)$.
        \item \textit{Copeland's rule III}. Define $u(x)=|U(x)|$. The final decision is formed by the alternatives with the lowest $u(x)$.
    \end{enumerate}
